# Supplementary material for: Do Neural Networks for Segmentation Understand Insideness?
Source: arXiv:2201.10664 source file (2022-01-25)
Supplement: Supplementary file 1 [file appendix1.tex]

\section{Formal Definitions About Insideness Problem} \label{Definitions}

Here we give formal definitions of basic notions used in this paper. 
We referred to the related definitions in the field of digital geometry~\cite{KR04} and in the book ``Perceptrons"~\cite{MP69,MP88}, 
but sometimes simplified or modified them for making the definitions most suitable for our purposes.

%%%% major modification 2/4 on Dec 19 by Tomotake %%%%
As in the main body of the paper, we refer to the matrix representation $\boldsymbol{X}\in \{0,1\}^{M\times N}$ as the image and to $X_{n,m}$ as the pixel in position $(n,m)$. 
 ${\mathtt F}_{ \boldsymbol{X} } = \{ X_{m,n}  = 1\}$ denotes the set of pixels in $\boldsymbol{X}$ with value 1.
We consider the so-called 4-adjacency for 1s and the so-called 8-adjacency for 0s. 
%%%% major modification 2/4 on Dec 19 by Tomotake %%%%

%%%% major modification 2/4 on Dec 19 by Tomotake%%%%
%\begin{dfn}
%When considering the matrix representation $\boldsymbol{X}\in \{0,1\}^{M\times N}$ of a black and white image, we slightly abuse notation and refer to $\boldsymbol{X}$ as the image and to $X_{n,m}$ as the pixel in position $(n,m)$, where we assume $(1,1)$ is the upper left corner of the image.
%\end{dfn}
%%%% major modification 2/4 on Dec 19 by Tomotake %%%%

\begin{dfn}[Border of an image] 
We refer to the border of an image $\boldsymbol{X}$ as the set of pixels $X_{n,m}$ such that $m = 1, m = M, n = 1$ or $n = N$. 
\end{dfn}

%%%% major modification 3/4 on Dec 19 by Tomotake %%%%
\begin{dfn}[digital Jordan curve]
Let ${\boldsymbol{X}} \in \{0,1\}^{M\times N}$ for some $N,M\geq 3$, and let  $c = ({\mathtt s}_{0}, {\mathtt s}_{1}, \ldots, {\mathtt s}_{L})$ for some $L \ge 8$ 
be a sequence of pixels in $\boldsymbol{X}$ such that they all have value 1. We call $c$ a digital Jordan curve in $\boldsymbol{X}$ if the following five conditions are satisfied:
\begin{enumerate}
\item ${\mathtt s}_{0} = {\mathtt s}_{L}$. \label{JCC1}
\item For any $i \in \{ 0, \ldots, L-1  \}$, pixels ${\mathtt s}_{i}$ and ${\mathtt s}_{i+1}$ are 4-adjacent. \label{JCC2}
\item It holds ${\mathtt s}_{i} \neq {\mathtt s}_{j}$ for all $i\neq j$ except for $0$ and $L$. \label{JCC3}
\item For any $i \in \{ 0, \ldots, L-1  \}$, ${\mathtt s}_{i}$ has no 4-adjacent pixel with value 1 in $\mathtt{F}_{\boldsymbol{X}} \setminus \{ {\mathtt s}_{0}, {\mathtt s}_{1}, \ldots, {\mathtt s}_{L-1} \}$. \label{JCC4}
\item For each $i \in \{ 0, \ldots, L-1  \}$, ${\mathtt s}_{i}$, there exist exactly two other pixels in $\{ {\mathtt s}_{0}, {\mathtt s}_{1}, \ldots, {\mathtt s}_{L-1} \}$ that are 4-adjacent to ${\mathtt s}_i$.    
\end{enumerate}
\end{dfn}

Note that conditions \ref{JCC1} and \ref{JCC2}  means the curve is closed, condition \ref{JCC3} means it doesn't have self-intersection or self-touching, condition \ref{JCC4} means it is isolated, and the last condition  means the ``thickness" of the curve is unitary. 
\begin{dfn}[inside region and outside region of an image]
Let $\boldsymbol{X} \in \{0,1\}^{M \times N}$ and suppose that ${\mathtt F}_{{\boldsymbol{X}}}$ is a digital Jordan curve in ${\boldsymbol{X}}$ which does not contain the border of $\boldsymbol{X}$. We define the outside region of ${\boldsymbol{X}}$ as the set of all pixels $\mathtt{v}_0$  in $\boldsymbol{X}$ with value 0 such that there exists a sequence of 0-value pixels starting from $\mathtt{v}_0$, 
\begin{align}
(\mathtt{v}_0, \mathtt{v}_{1}, \mathtt{v}_{2}, \dots, \mathtt{v}_{L}), 
\end{align}
where pixels $\mathtt{v}_{i}$ and $\mathtt{v}_{i+1}$ are 8-adjacent, 
and $\mathtt{v}_{L}$ is the border of the image $\boldsymbol{X}$.

We define the inside region of ${\boldsymbol{X}}$ as the set of pixels with value 0 that are not in the outside region.
\end{dfn}
%%%% major modification 4/4 on Dec 19 by Tomotake %%%%

%%%% major modification 4/4 on Dec 19 by Tomotake %%%%
%\begin{dfn}[inside region and outside region of an image]
%Let $\boldsymbol{X} \in \{0,1\}^{M \times N}$ and suppose that ${\mathtt F}_{{\boldsymbol{X}}}$ (the set of pixels in $\boldsymbol{X}$ with value 1) is a digital Jordan curve in ${\boldsymbol{X}}$ which does not contain the border of $\boldsymbol{X}$. We define the outside region of ${\boldsymbol{X}}$ as the set of all pixels $\mathtt{v}_0$  in $\boldsymbol{X}$ with value 0 such that there exists a sequence of 0-value pixels starting from $\mathtt{v}_0$, 
%\begin{align}
%(\mathtt{v}_0, \mathtt{v}_{1}, \mathtt{v}_{2}, \dots, \mathtt{v}_{L}), 
%\end{align}
%where pixels $\mathtt{v}_{i}$ and $\mathtt{v}_{i+1}$ have a common vertex, 
%and $\mathtt{v}_{L}$ is the border of the image $\boldsymbol{X}$.
%
%We define the inside region of ${\boldsymbol{X}}$ as the set of pixels with value 0 that are not in the outside region.
%\end{dfn}
%%%% major modification 4/4 on Dec 19 by Tomotake %%%%
