# Supplementary material for: Do Neural Networks for Segmentation Understand Insideness?
Source: arXiv:2201.10664 source file (2022-01-25)
Supplement: Supplementary file 2 [file appendix3.tex]

\section{Details for Proof of Theorem \ref{Theorem1}} \label{AppThm1}
Weights and biases are determined as follows:
$\boldsymbol{w}^{(2)}=\boldsymbol{ {\it 1}}_{1 \times N} \in \mathbb{R}^{1 \times N}$, 
$\boldsymbol{B}_{r}^{(2)} \in \mathbb{R}^{M \times N} $ is defined by 
\begin{align}
(B_{r}^{(2)})_{m,n} = 
    \begin{cases}
       -(2 u -\frac{1}{2}) &\quad \text{if } r = 3u +1, \\
       -2 u &\quad\text{if } r = 3u +2, \\
       -(2 u +\frac{1}{2})  &\quad \text{if } r = 3u +3, \\ 
     \end{cases}  \label{def_b}
\end{align}
for all $1 \leq m \leq M$ and $1 \leq n \leq N$ where $u \in \mathbb{N}_{0}$,
$\boldsymbol{w}^{(3)} \in \mathbb{R}^{1\times 1 \times C'}$ is defined by 

\begin{align}
w_{r}^{(3)} = 
     \begin{cases}
       -2 &\quad\text{if } r \equiv 1 \pmod{3},\\
       4 &\quad\text{if } r \equiv 2 \pmod{3}, \\
       -2 &\quad\text{if } r \equiv 3 \pmod{3}, \\ 
     \end{cases} 
\end{align}
and $\boldsymbol{B}^{(3)} = \boldsymbol{ {\it 1}}_{M \times N} \in \mathbb{R}^{M \times N}$. \\

We had $\boldsymbol{ {\it 1}}_{1 \times N} \cdot \vec{H}^{(1)}_{m, n}=\vec{X}_{m, n} \cdot \vec{X}_{m+1, n}.$ Therefore,
\begin{align}
\mathrm{H}^{(2)}_{m,n,r} = \boldsymbol{ {\it 1}}_{1 \times N} \cdot \vec{H}^{(1)}_{m, n} +  ({B}_{r}^{(2)})_{m,n} = \vec{X}_{m, n} \cdot \vec{X}_{m+1, n} + ({B}_{r}^{(2)})_{m,n}.
\end{align}

Next, notice that for each $r=3u+i$ with $i\in\{1,2,3\},$ there exists $v \in \mathbb{Z}$ such that it holds $\vec{X}_{m, n} \cdot \vec{X}_{m+1, n} = 2u +  v$.
Then, 
\begin{align}
\mathrm{H}_{m, n, r}^{(2)} = 
     \begin{cases}
       \left[v + \frac{1}{2}\right]_{+} &\quad \text{if } r = 3u +1 \\
       [v]_{+} &\quad\text{if } r = 3u +2 \\
       \left[v - \frac{1}{2} \right]_{+} &\quad \text{if } r =3u +3,  
     \end{cases} 
\end{align}
and summing these three equations we can see that
\begin{align}
    -2 \mathrm{H}^{(2)}_{m, n, 3 u + 1} + 4 \mathrm{H}^{(2)}_{m, n, 3 u + 2} -2 \mathrm{H}^{(2)}_{m, n, 3u + 3} = 
    \begin{cases}
    -1  &\quad\text{if } v = 0,\\
    0  &\quad\text{otherwise. }
    \end{cases} 
    \label{Eq: 2}
\end{align}

Lastly, by definition of the output layer we obtain
\begin{align}
\begin{split}
    Y_{m,n}
    &=\left[ \sum_{r = 1}^{3\left(\lfloor\frac{C}{2}\rfloor+1\right)} w_{r}^{(3)} \mathrm{H}_{m,n,r}^{(2)} + 1 \right]_{+}\\
    &=\left [\sum_{u = 0}^{\lfloor\frac{C}{2}\rfloor}\left (w^{(3)}_{3u+1} \mathrm{H}^{(2)}_{m,n,3u+1}+w^{(3)}_{3u+2} \mathrm{H}^{(2)}_{m,n,3u+2}+w^{(3)}_{3u+3} \mathrm{H}^{(2)}_{m,n,3u+3}\right) + 1 \right ]_{+}\\
    &= \left[\left (\sum_{u=0}^{\lfloor\frac{C}{2}\rfloor}-2 \mathrm{H}^{(2)}_{m, n, 3 u + 1} + 4 \mathrm{H}^{(2)}_{m, n, 3 u + 2} -2 \mathrm{H}^{(2)}_{m, n, 3 u + 3}\right ) +1 \right ]_{+}\\
    &=
     \begin{cases}
       0 &\quad\text{if } \vec{X}_{m, n} \cdot \vec{X}_{m+1, n} =  2u \quad \text{ for some } 0\leq u \leq \lfloor\frac{C}{2}\rfloor \\
       1 &\quad\text{otherwise. }
     \end{cases} 
\end{split}
\end{align}

By \textit{Lemma 1} and the fact that $\vec{X}_{m, n} \cdot \vec{X}_{m+1, n} \leq C$, we conclude that
\begin{align}
Y_{m,n} &=
\left \{
    \begin{array}{cll}
    0 & \text{if } \vec{X}_{m, n} \cdot \vec{X}_{m+1, n} \text{ is even} & \Leftrightarrow X_{m,n} \text{ is  outside}, \\
    1 & \text{if } \vec{X}_{m, n} \cdot \vec{X}_{m+1, n} \text{ is odd}    & \Leftrightarrow {X}_{m,n} \text{ is  inside}.
    \end{array}
\right.
\end{align}

\qed
