# Supplementary material for: Do Neural Networks for Segmentation Understand Insideness?
Source: arXiv:2201.10664 source file (2022-01-25)
Supplement: Supplementary file 3 [file appendix2.tex]

\section{Neural Network Representations of Boolean Operations} \label{Boolean}

In the Coloring Network, we use neural network representations (implementations) 
of Boolean NOT and Boolean AND as building blocks. 
Here we explain the details.

\subsection{Neural Network Representation of Boolean NOT} \label{AppFlip}

In addition to the normal notation $\neg$, 
we use $\mathrm{NOT}: \{0,1 \} \to \{0,1 \}$ to denote the Boolean NOT.
That is, 
\begin{align} 
\mathrm{NOT}(x) = \neg x = 
\left \{
\begin{array}{ll}
1 & \text{if } x = 0, \\
0 & \text{if } x = 1.
\end{array}
\right.
\end{align}
Like other functions, we use $\mathbf{NOT}$ to denote element-wise application of $\mathrm{NOT}$ to a vector or a matrix. We here show that this function can be represented by a neural network with rectified linear function.\\

Let  $x \in \{0,1\}$ and consider the neural network
$f^{ \mathrm{N}}(\cdot ; \boldsymbol{\theta})$ defined by 
\begin{align}
f^{ \mathrm{N}}(x ; \boldsymbol{\theta})  \coloneqq [wx + b]_{+} \in \{0,1\},
\end{align}
where $ \boldsymbol =   (w, b) \in \mathbb{R}^2$. It is easy to check that defining $\boldsymbol{\theta}=(-1,1)$, we obtain 
\[
f^{ \mathrm{N}}(x ; \boldsymbol{\theta_{ \mathrm{N}}})=NOT(x).
\]
We can then generalize to higher-order cases as follows. Let $\boldsymbol{X} \in \{0,1\}^{I \times J}$ and consider the neural network $\boldsymbol{F}^{ \mathrm{N}}(\cdot ; \boldsymbol{\varTheta})$ defined by
\[
\boldsymbol{F}^{ \mathrm{N}}(\boldsymbol{X} ; \boldsymbol{\varTheta}) 
\coloneqq [w\ast \boldsymbol{X} + \boldsymbol{B}]_{+}\in \mathbb{R}^{I \times J},
\]
where $\boldsymbol{\varTheta}=(w, \boldsymbol{B} )$. Setting  $\boldsymbol{\varTheta}_{\mathrm{N}}=(-1,\boldsymbol{{\it 1}}_{I \times J})$, we obtain
$\boldsymbol{F}^{\mathrm{N}}(\boldsymbol{X}; \boldsymbol{\varTheta}_{\mathrm{N}}) = \mathbf{NOT}(\boldsymbol{X})$.

\subsection{Neural Network Representation of Boolean AND } \label{NNRepresentation}

In addition to the normal operator notation $\wedge$, 
we use $\mathrm{AND}: \{0,1 \} \times \{0,1 \} \to \{0,1 \}$ to denote the Boolean AND.
That is, 
\begin{align} 
\mathrm{AND}(x_{1}, x_{2}) = x_{1} \wedge x_{2} = x_{1} \cdot x_{2}  = 
\left \{
\begin{array}{ll}
1 & \text{if } x_{1} = 1, x_{2} = 1\\
0 & \text{otherwise}. 
\end{array}
\right.
\end{align}
Here, $\mathbf{AND}$ denotes element-wise application of $\mathrm{AND}$ to vectors or matrices. This can also be implemented by a neural network with rectified linear activation function as shown below.\\

Let  $x_{1}, x_{2} \in \{0,1\}$ and consider the neural network
$f^{\mathrm{A}}(\cdot , \cdot ; \boldsymbol{\theta})$ defined by 
\[
y =f^{\mathrm{A}}(x_{1} , x_{2} ; \boldsymbol{\theta}) \coloneqq [\boldsymbol{w} \cdot [x_{1} , x_{2}]^{\top} + b]_{+}\in \{0,1\},
\]
where $\boldsymbol{\theta} =   (\boldsymbol{w}, b)$. It is easy to verify that setting $\boldsymbol{\theta}_{\mathrm{A}}=(\boldsymbol{{\it 1}}_{2}, -1)$ we obtain
\[
f^{\mathrm{A}}(x_{1}, x_{2} ; \boldsymbol{\theta}_{\mathrm{A}}) = \mathrm{AND}(x_{1} , x_{2})
\]

As in the case of the Boolean NOT, we can generalize this function to higher order cases, but before doing so, we introduce some notation.

Informally speaking, we use $\boldsymbol{A} \boxplus \boldsymbol{B}$ to denote a tensor made by ``stacking" a matrix $ \boldsymbol{B}$ ``behind" a matrix $\boldsymbol{A}$. 
Formal definition is as follows. 
Consider $\boldsymbol{A} = [A_{i, j}] \in \mathbb{R}^{I \times J}$ 
and $ \boldsymbol{B} = [B_{i, j}] \in \mathbb{R}^{I \times J}$. 
We define a tensor $\boldsymbol{A} \boxplus \boldsymbol{B} = [(\boldsymbol{A} \boxplus \boldsymbol{B})_{i, j, k }] \in \mathbb{R}^{I \times J \times 2}$ 
by the following equations: 
\begin{align}
(\boldsymbol{A} \boxplus \boldsymbol{B})_{i, j, 1 } & \coloneqq A_{i, j},  \\
(\boldsymbol{A} \boxplus \boldsymbol{B})_{i, j, 2 } & \coloneqq B_{i, j},  
\end{align}
for all $1\leq i \leq I$ and $1\leq j \leq J$.

We can then extend the neural network $f^{\mathrm{A}}$ as follows. Let $\boldsymbol{X}_{1},\boldsymbol{X}_{2} \in \{0,1\}^{I \times J}$ 
and consider the neural network $\boldsymbol{F}^{\mathrm{A}}(\cdot , \cdot ; \boldsymbol{\varTheta})$ defined by
\[ \boldsymbol{F}^{\mathrm{A}}(\boldsymbol{X}_{1} , \boldsymbol{X}_{2} ; \boldsymbol{\varTheta})  \coloneqq  [\boldsymbol{w} \ast  (\boldsymbol{X}_{1} \boxplus \boldsymbol{X}_{2}) + \boldsymbol{B}  ]_{+}\in \mathbb{R}^{I \times J},
\]
where  
$\boldsymbol{\varTheta} = (\boldsymbol{w},  \boldsymbol{B})$. Setting $\boldsymbol{\varTheta}_{\mathrm{A}}= ([1,1], - \boldsymbol{{\it 1}}_{I \times J})$ we obtain

\[
\boldsymbol{F}^{\mathrm{A}}(\boldsymbol{X}_{1} , \boldsymbol{X}_{2} ; \boldsymbol{\varTheta}_{\mathrm{A}}) = \mathbf{AND}(\boldsymbol{X}_{1} , \boldsymbol{X}_{2}) = \boldsymbol{X}_{1}  \odot  \boldsymbol{X}_{2}.
\]
where $\odot$ expresses the Hadamard porduct (element-wise product) of two matrices.
