# Supplementary material for: Do Neural Networks for Segmentation Understand Insideness?
Source: arXiv:2201.10664 source file (2022-01-25)
Supplement: Supplementary file 5 [file dilation_vis_supp.tex]

\begin{figure}[t!]
  \footnotesize
  \centering
  \begin{tabular}{cc}
     \multicolumn{2}{c}{\bf Examples of Feature Maps  of the Dilated Conv. DNN }\\
     [0.1in]
     \includegraphics[width=0.47\textwidth]{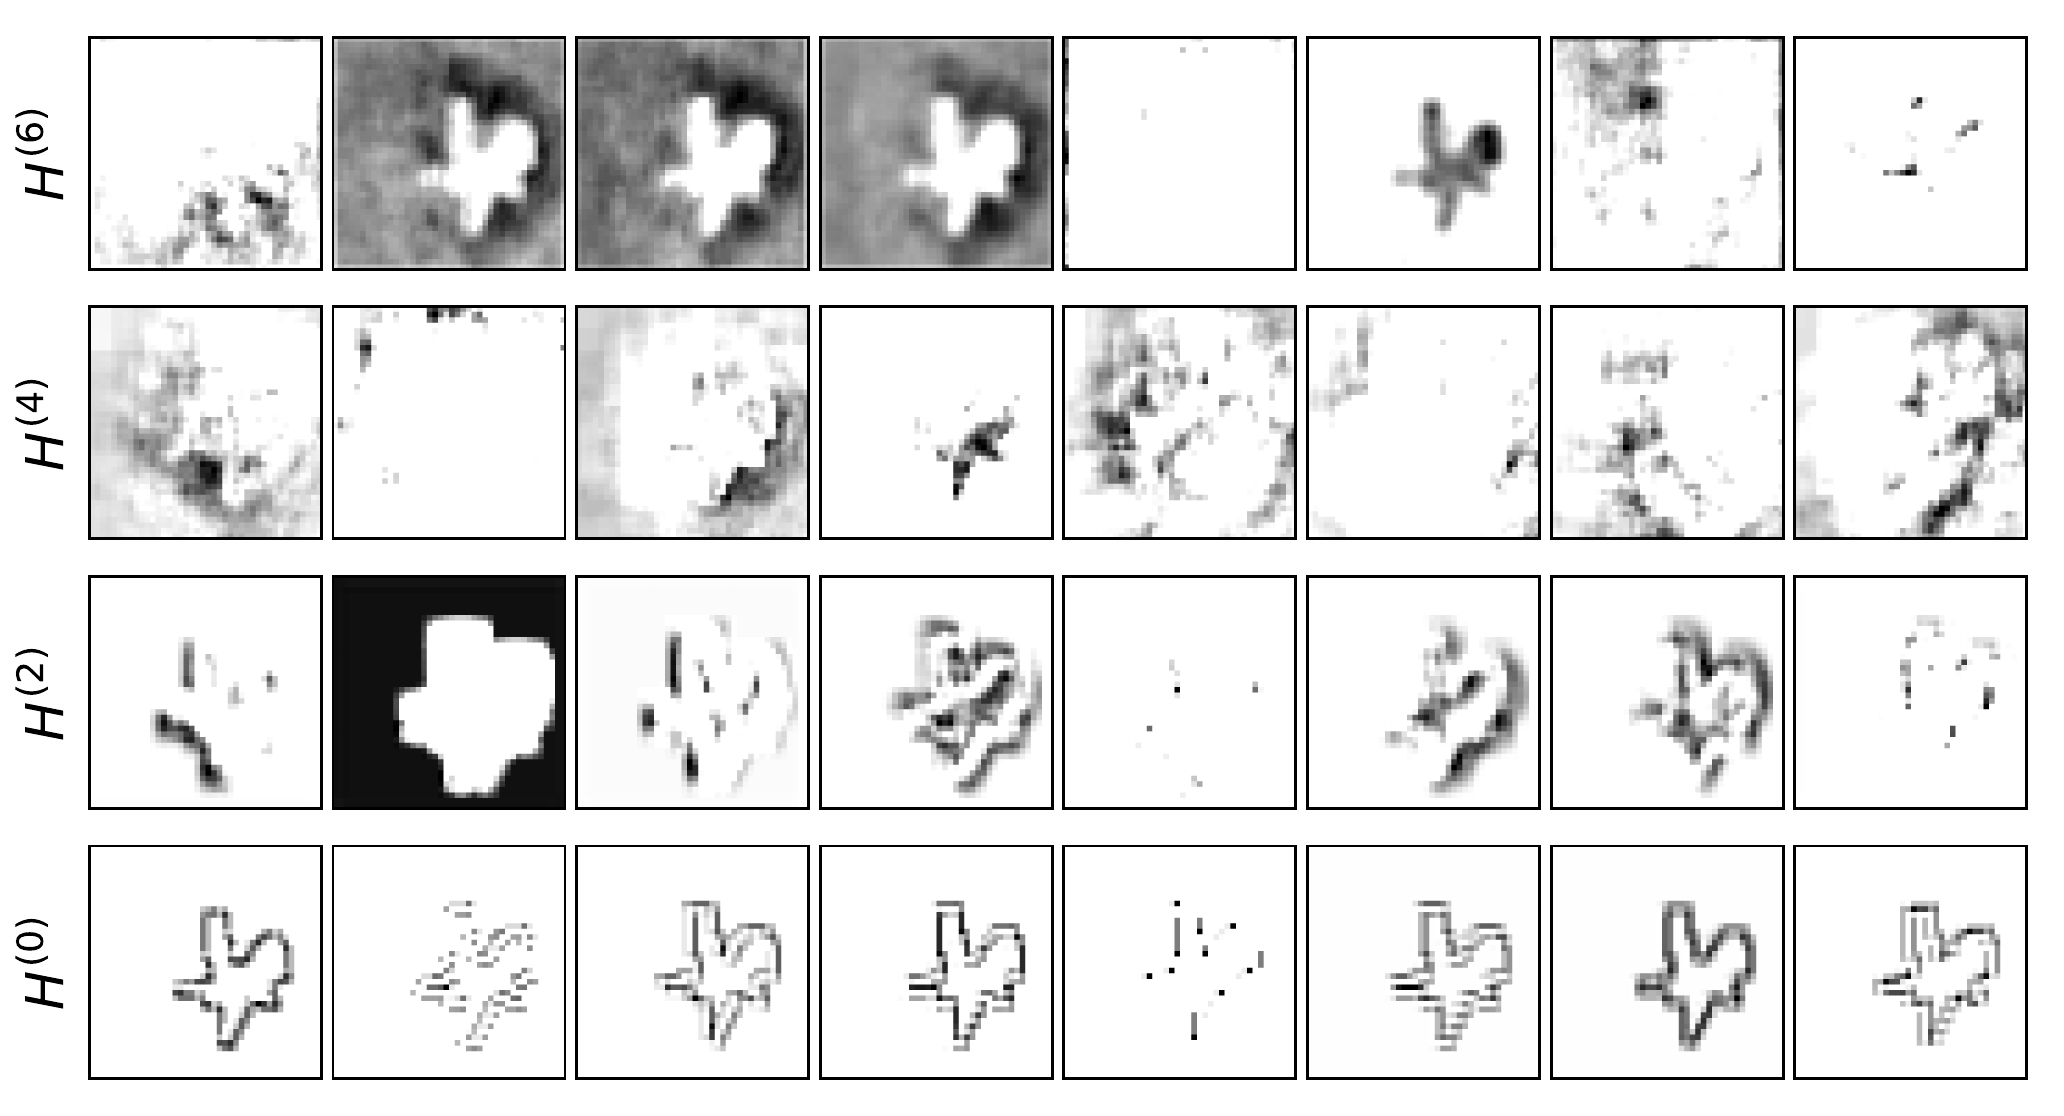} &
          \includegraphics[width=0.47\textwidth]{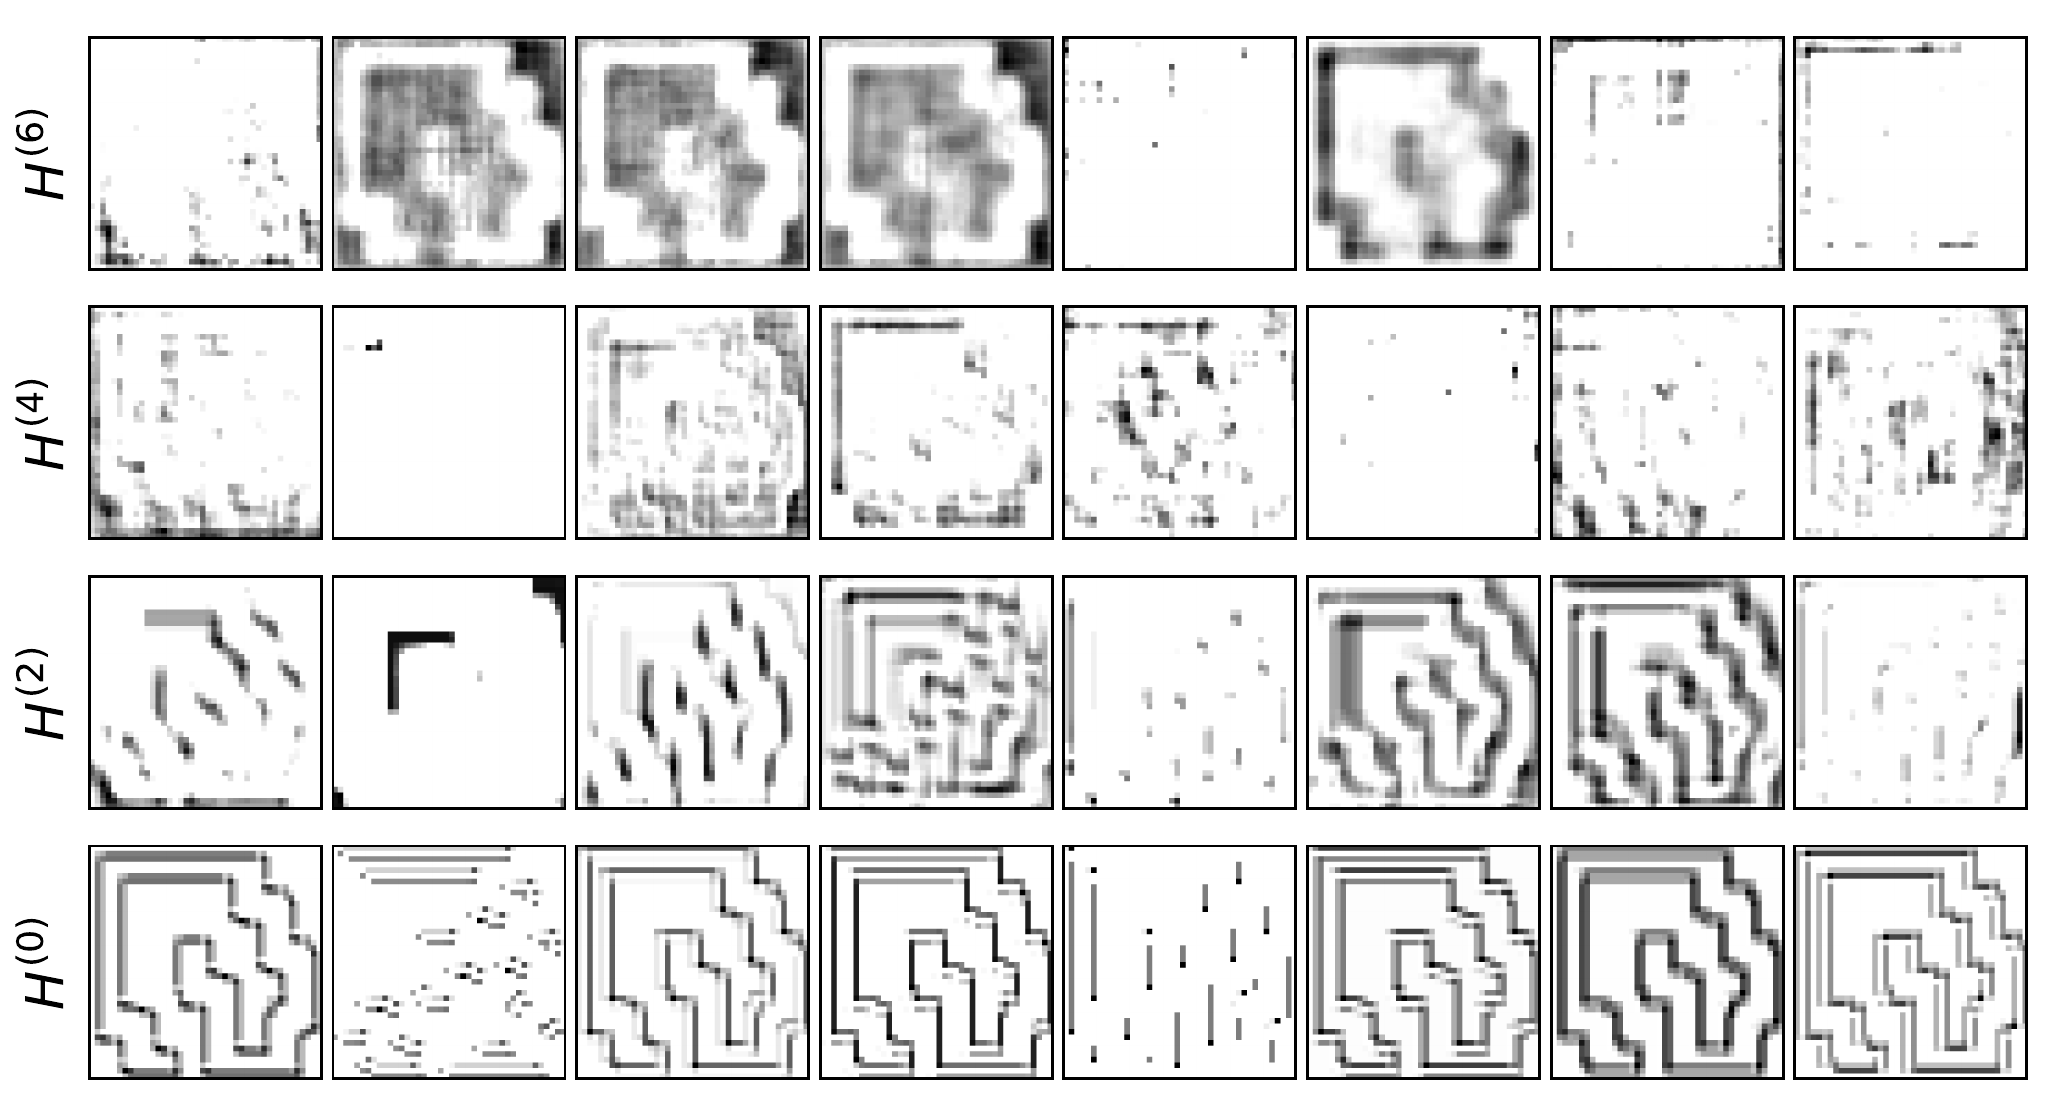}\\
          [0.1in]
          \includegraphics[width=0.47\textwidth]{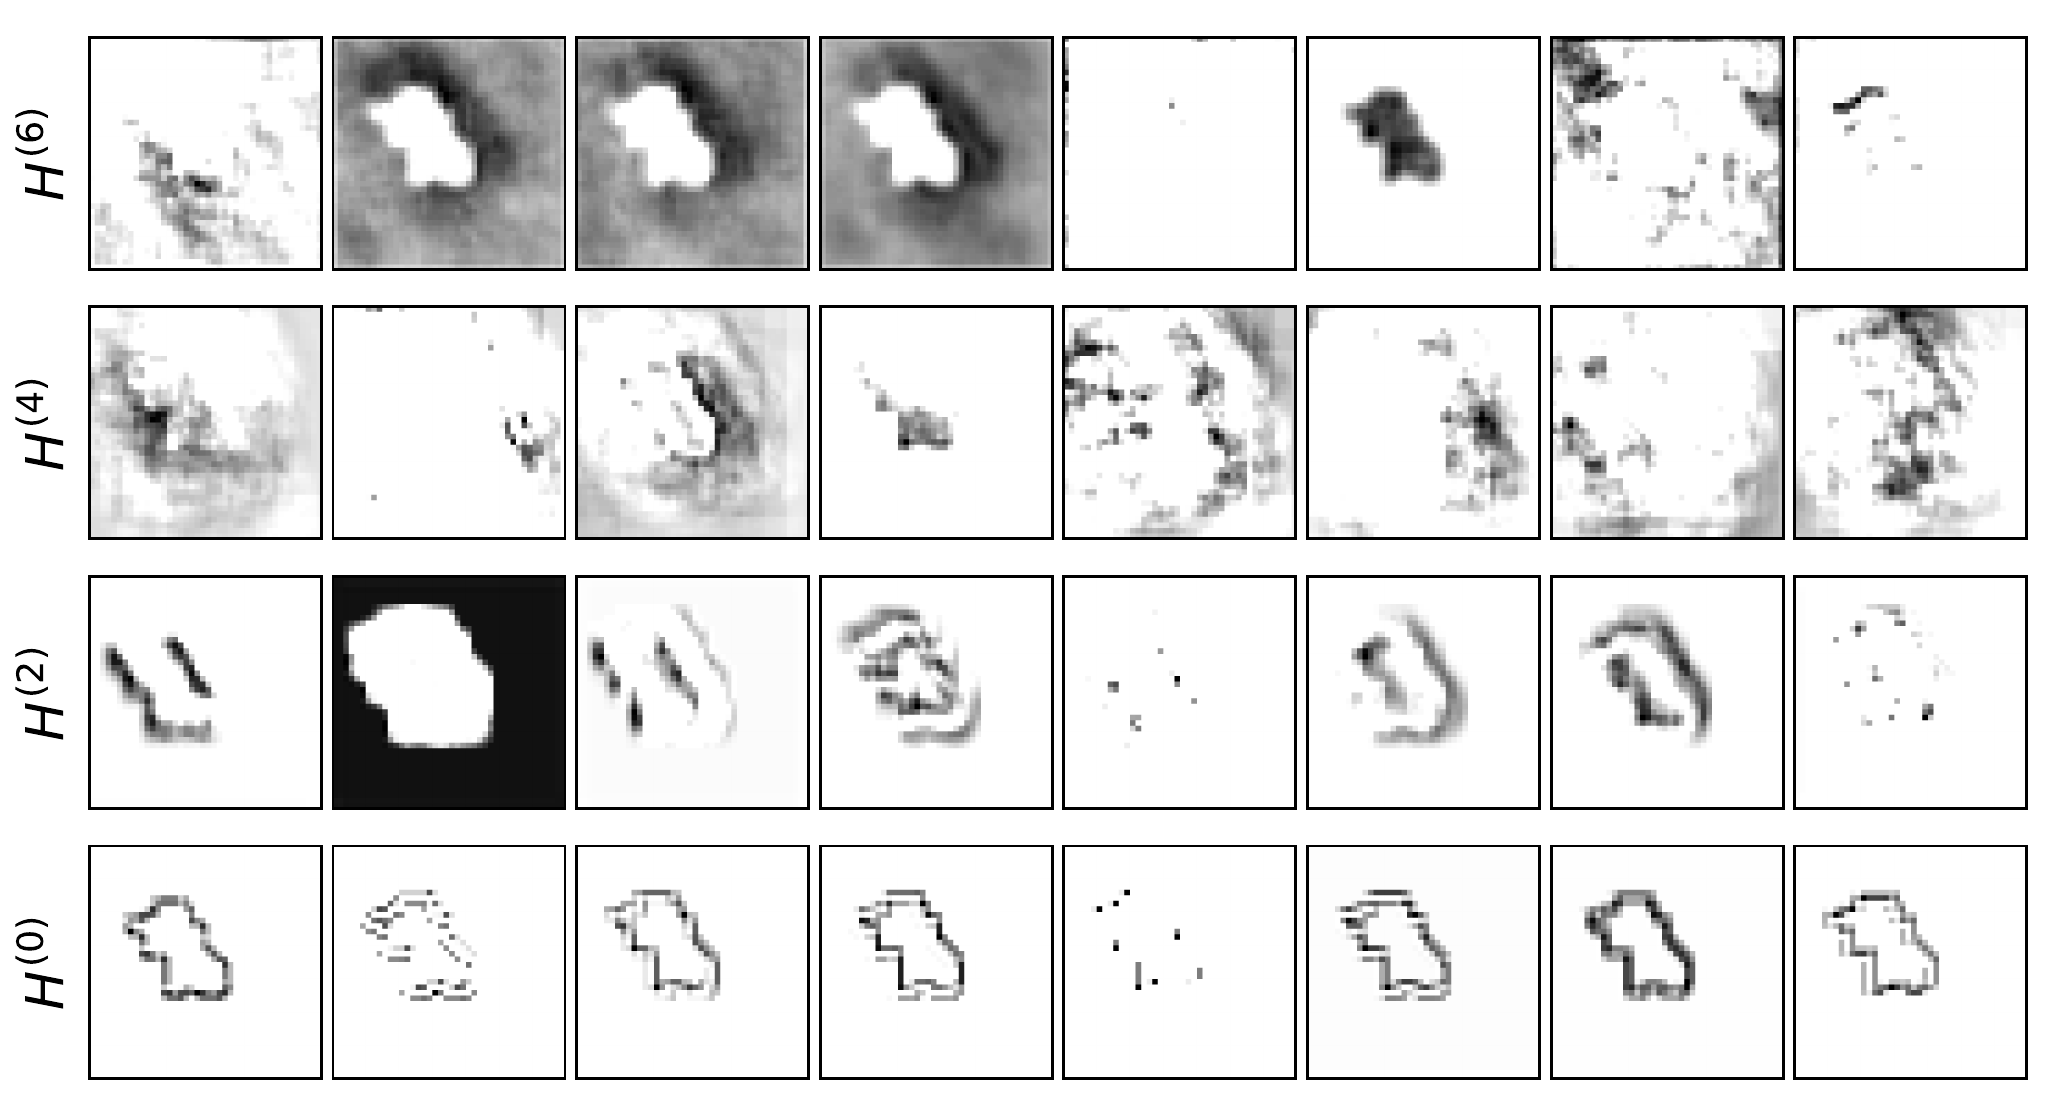} & 
          \includegraphics[width=0.47\textwidth]{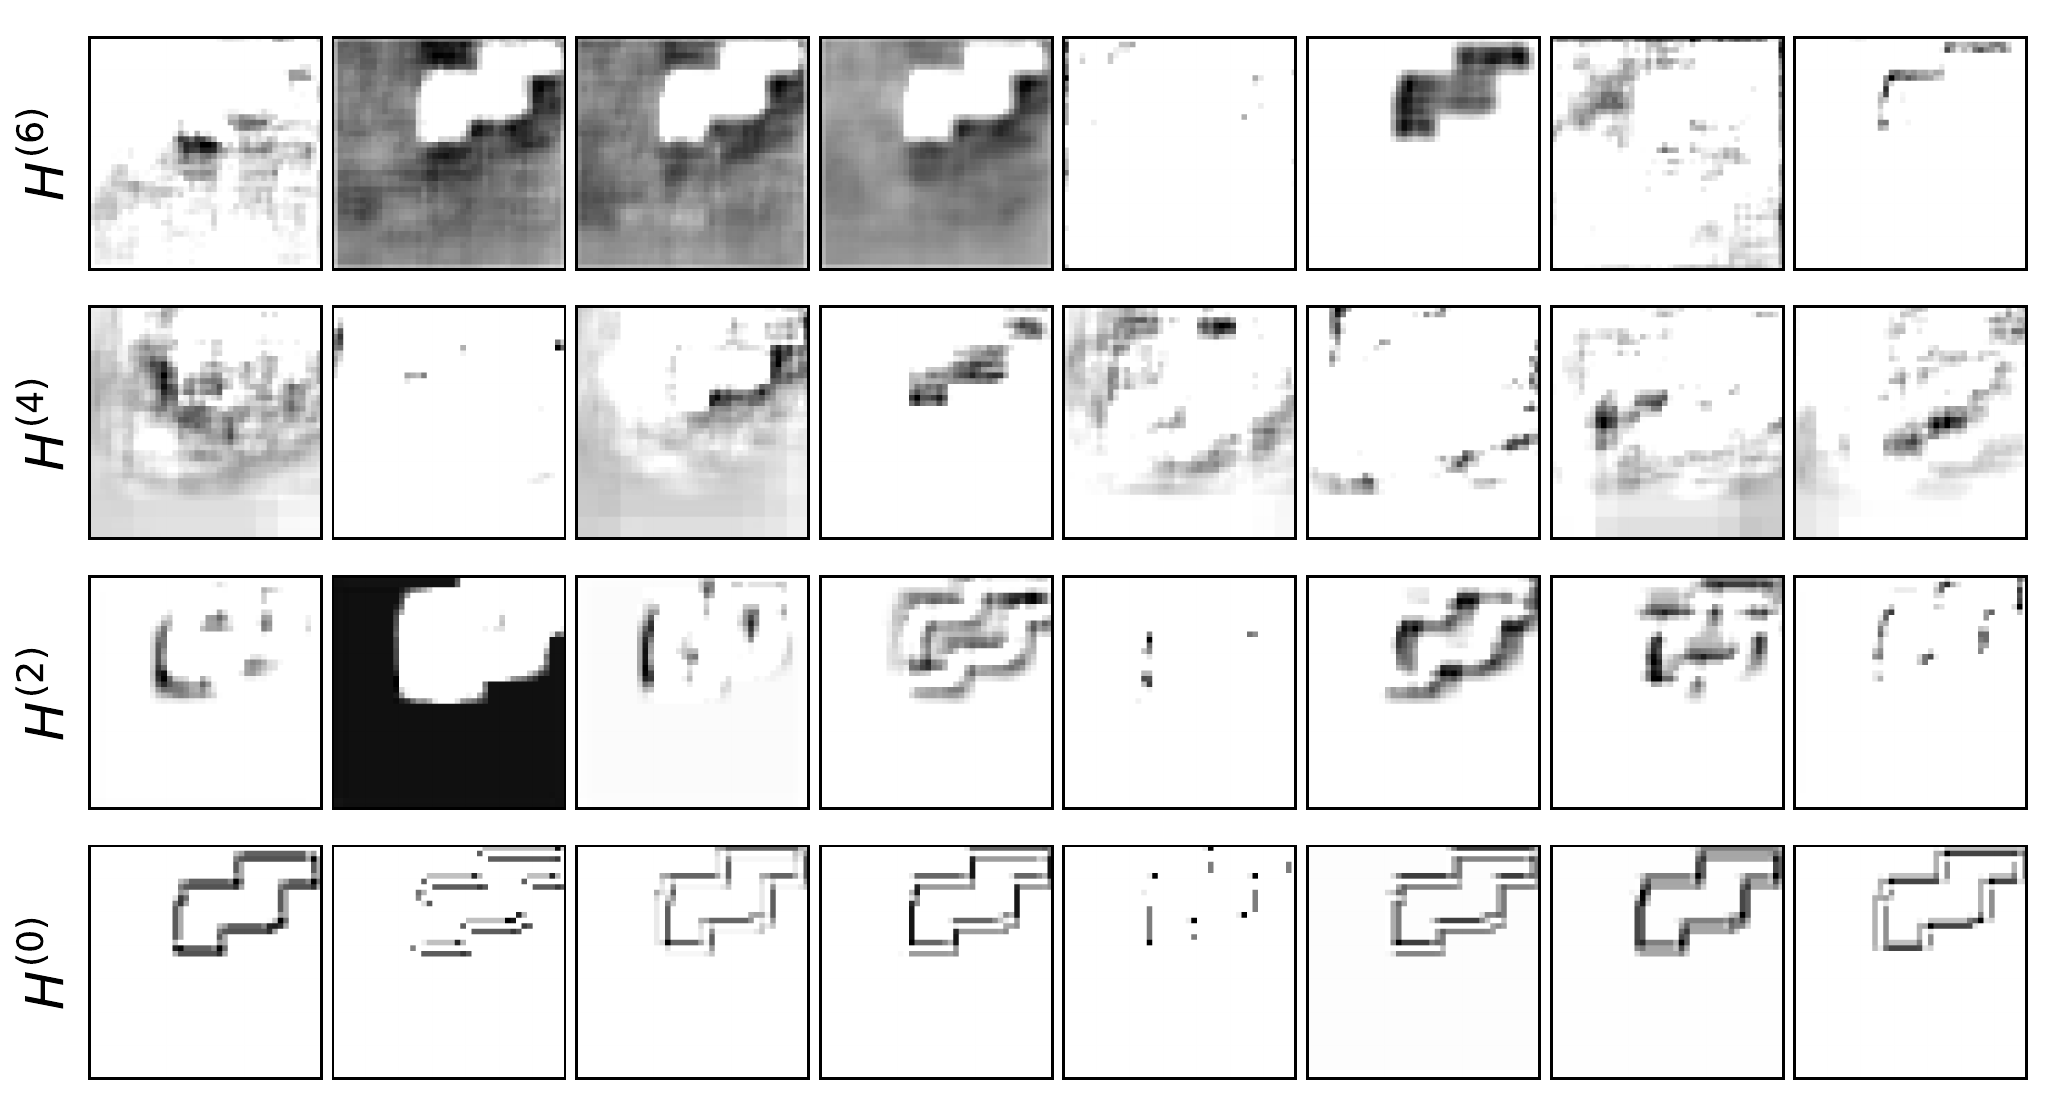}
  \end{tabular}
\caption{\emph{Visualization of the Feature Maps of the DNN with Dilated Convolutions.} We display several feature maps at different layers (each row in each block is a different layer). We can see that the first layers detect lower level features such as edges with specific orientations, while the later layers capture long-range dependencies of the curve relative to insideness.}
\label{figDilateionVis}
\end{figure}
