# Supplementary material for: Do Neural Networks for Segmentation Understand Insideness?
Source: arXiv:2201.10664 source file (2022-01-25)
Supplement: Supplementary file 7 [file quantiative2_supp.tex]

\begin{figure}[t]
  \footnotesize
        \includegraphics[width=0.45\textwidth]{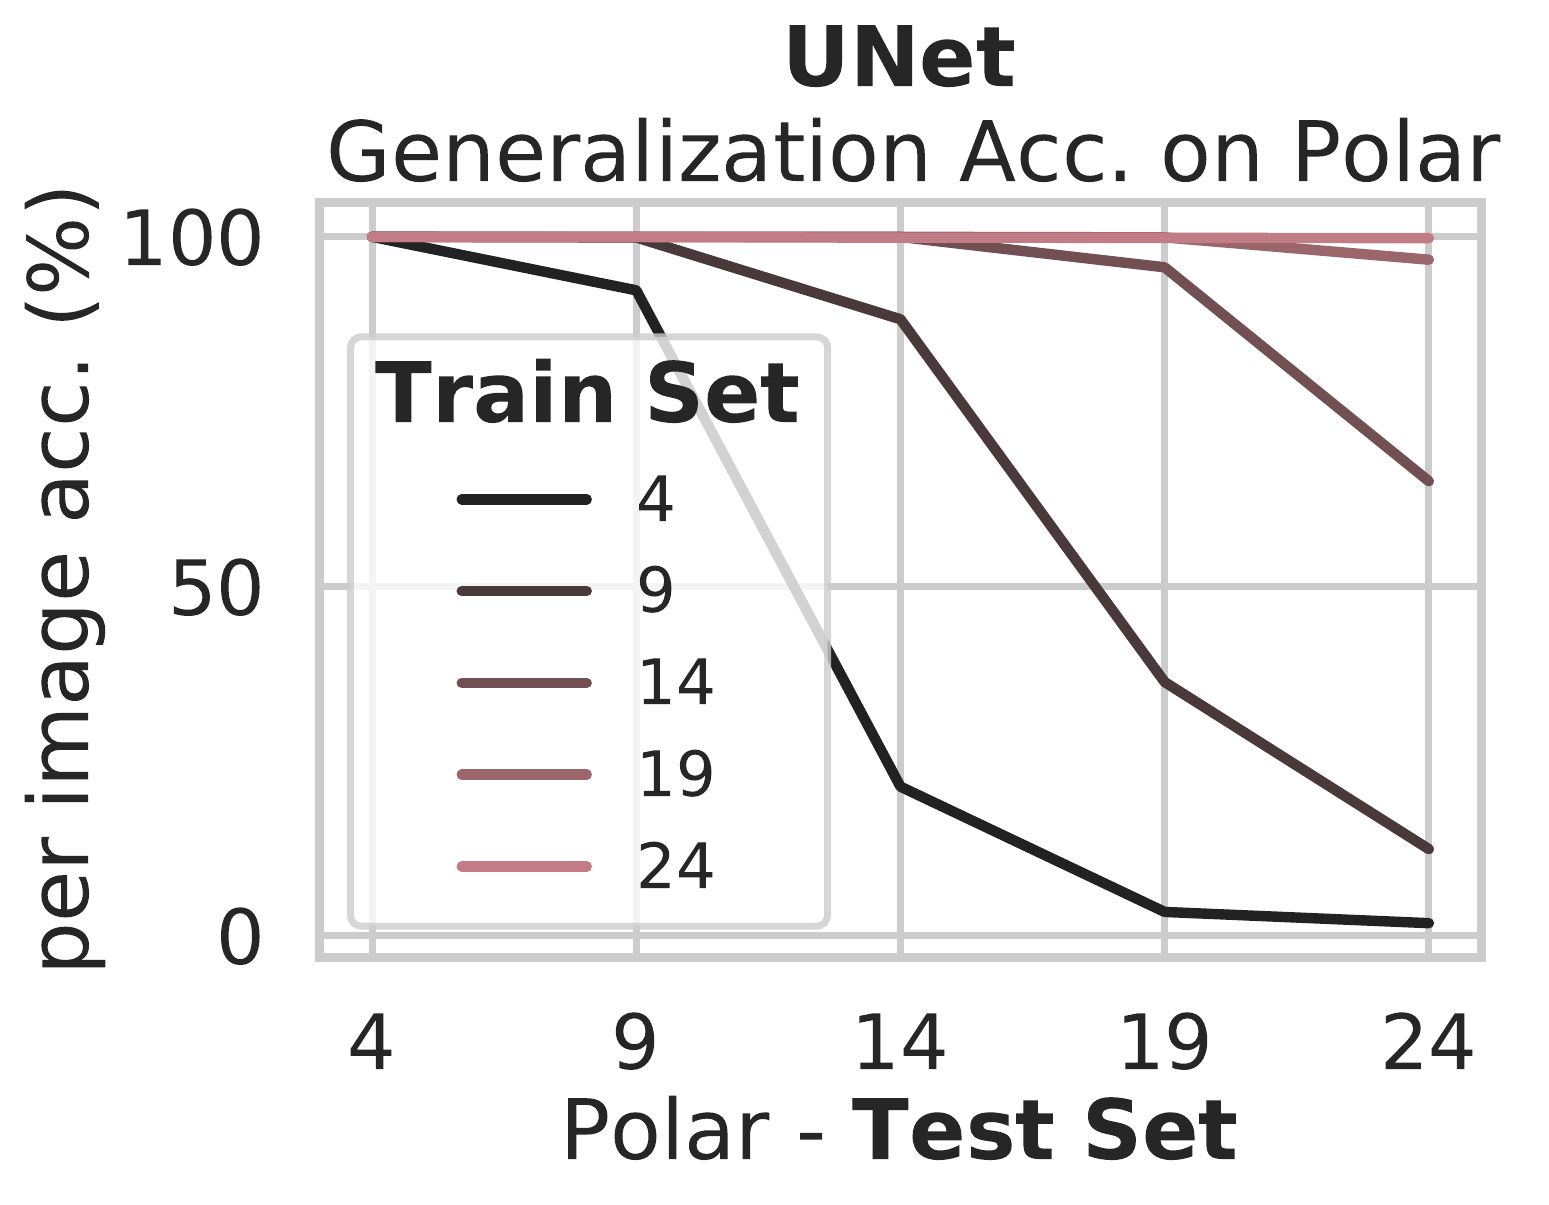}
\caption{\emph{Training Accuracy in the Polar Dataset.} Intra-dataset evaluation using (a) per pixel accuracy and (b) per image accuracy. }
\label{resSuppQuant2}
\end{figure}
